# Supplementary material for: RIFT: Entropy-Optimised Fractional Wavelet Constellations for Ideal Time-Frequency Estimation
Source: arXiv:2501.15764 source file (2026-04-01)
Supplement: Supplementary file 1 [file supp.tex]

\input{preamble}

\usepackage{xr}
\externaldocument{full}

\begin{document}

\syncfromfull{equation}{x_6}
\syncfromfull{figure}{fig:montage_main}

\setcounter{table}{1}

\input{supp_body}

\end{document}
